# Supplementary material for: System of Agentic AI for the Discovery of Metal-Organic Frameworks
Source: arXiv:2504.14110 source file (2025-04-18)

# checkCIF/PLATON report

Structure factors have been supplied for datablock(s) sm_621b

THIS REPORT IS FOR GUIDANCE ONLY. IF USED AS PART OF A REVIEW PROCEDURE FOR PUBLICATION, IT SHOULD NOT REPLACE THE EXPERTISE OF AN EXPERIENCED CRYSTALLOGRAPHIC REFEREE.

No syntax errors found. CIF dictionary Interpreting this report

# Datablock: sm_621b

---

Bond precision: C-C = 0.0045 A Wavelength=1.54178

| | | | |
|---|---|---|---|
| Cell: | a=22.0122(10) | b=18.1336(8) | c=10.5378(5) |
| | alpha=90 | beta=90 | gamma=90 |
| Temperature: | 200 K | | |

| | Calculated | Reported |
|---|---|---|
| Volume | 4206.3(3) | 4206.3(3) |
| Space group | P n a 21 | P n a 21 |
| Hall group | P 2c -2n | P 2c -2n |
| Moiety formula | C24 H32 N2 O15 Zn4 [+ solvent] | C24 H32 N2 O15 Zn4 |
| Sum formula | C24 H32 N2 O15 Zn4 [+ solvent] | C24 H32 N2 O15 Zn4 |
| Mr | 850.08 | 849.99 |
| Dx,g cm-3 | 1.342 | 1.342 |
| Z | 4 | 4 |
| Mu (mm-1) | 3.066 | 3.066 |
| F000 | 1720.0 | 1720.0 |
| F000' | 1699.81 | |
| h,k,lmax | 26,22,12 | 26,21,12 |
| Nref | 7911[ 4187] | 7317 |
| Tmin,Tmax | 0.832,0.858 | 0.607,0.753 |
| Tmin' | 0.736 | |

Correction method= # Reported T Limits: Tmin=0.607 Tmax=0.753
AbsCorr = NONE

Data completeness= 1.75/0.92 Theta(max)= 69.561

R(reflections)= 0.0221( 7189)    wR2(reflections)= 0.0577( 7317)

S = 1.100    Npar= 411

---

The following ALERTS were generated. Each ALERT has the format
**test-name_ALERT_alert-type_alert-level.**
Click on the hyperlinks for more details of the test.

---

### Alert level C

```
STRVA01_ALERT_4_C           Flack test results are ambiguous.
           From the CIF: _refine_ls_abs_structure_Flack    0.490
           From the CIF: _refine_ls_abs_structure_Flack_su    0.020
PLAT220_ALERT_2_C NonSolvent   Resd 1  C   Ueq(max)/Ueq(min) Range        4.7 Ratio
PLAT242_ALERT_2_C Low    'MainMol' Ueq as Compared to Neighbors of       N1SA Check
PLAT242_ALERT_2_C Low    'MainMol' Ueq as Compared to Neighbors of       N1SB Check
PLAT911_ALERT_3_C Missing FCF Refl Between Thmin & STh/L=    0.600         52 Report
                1 21  0,   2  0  0,   3  5  0,   4  0  0,   4  3  0,   4 21  0,
                5 21  0,   6  2  0,   6  7  0,   6 21  0,   9 20  0,  16 17  0,
               20  0  0,  21  9  0,  21 11  0,  22  0  0,  22  1  0,  22  3  0,
               23 10  0,  24  4  0,  24  7  0,  26  2  0,  20 13  1,  21  5  1,
               22  7  1,   2 20  2,   3  1  2,  26  1  2,   1 21  3,   8  0  3,
                8 17  3,  19 10  3,  24  2  3,   0 20  4,   4 20  4,   0  3  5,
                0 19  5,   3 19  5,   4 18  5,   4 18  6,   5 16  6,   8 15  6,
                0 12  8,   1 15  9,   2 15  9,   5 11  9,  12  9  9,   6  2 10,
                0  2 12,   0  4 12,   5  4 12,   8  1 12,
```

---

### Alert level G

```
PLAT004_ALERT_5_G Polymeric Structure Found with Maximum Dimension          3 Info
PLAT171_ALERT_4_G The CIF-Embedded .res File Contains EADP Records          1 Report
PLAT606_ALERT_4_G Solvent Accessible VOID(S) in Structure ........          ! Info
PLAT720_ALERT_4_G Number of Unusual/Non-Standard Labels ..........         43 Note
              O1SB    O1SA    C00K    H6BA    H6BB    H6BC    H5BA    H5BB
              H5BC    N1SA    N1SB    C1SB    H1SB    H6CA    H6CB    H6CC
              H5CA    H5CB    H5CC    C1SA    H1SA    H5AA    H5AB    H5AC
              H4AA    H4AB    H4AC    C3SB    H3SA    H3SB    H3SC    C2SA
              H2SA    H2SB    H2SC    C2SB    H2SD    H2SE    H2SF    C3SA
              H3SD    H3SE    H3SF
PLAT794_ALERT_5_G Tentative Bond Valency for Zn1       (II)      .       2.09 Info
PLAT794_ALERT_5_G Tentative Bond Valency for Zn2       (II)      .       2.04 Info
PLAT794_ALERT_5_G Tentative Bond Valency for Zn3       (II)      .       2.05 Info
PLAT794_ALERT_5_G Tentative Bond Valency for Zn4       (II)      .       2.09 Info
PLAT868_ALERT_4_G ALERTS Due to the Use of _smtbx_masks Suppressed          ! Info
PLAT912_ALERT_4_G Missing # of FCF Reflections Above STh/L=  0.600         43 Note
PLAT913_ALERT_3_G Missing # of Very Strong Reflections in FCF ....          1 Note
                2  0  0,
PLAT933_ALERT_2_G Number of HKL-OMIT Records in Embedded .res File          3 Note
               -1 -1 -2,   1  1  2,  -3 -1 -1,
PLAT969_ALERT_5_G The 'Henn et al.' R-Factor-gap value ...........      3.025 Note
              Predicted wR2: Based on SigI**2  1.91 or SHELX Weight  5.24
PLAT978_ALERT_2_G Number C-C Bonds with Positive Residual Density.          0 Info
PLAT992_ALERT_5_G Repd & Actual _reflns_number_gt Values Differ by          3 Check
```

---

```
  0 ALERT level A = Most likely a serious problem - resolve or explain
  0 ALERT level B = A potentially serious problem, consider carefully
  5 ALERT level C = Check. Ensure it is not caused by an omission or oversight
 15 ALERT level G = General information/check it is not something unexpected

  0 ALERT type 1 CIF construction/syntax error, inconsistent or missing data
  5 ALERT type 2 Indicator that the structure model may be wrong or deficient
  2 ALERT type 3 Indicator that the structure quality may be low
  6 ALERT type 4 Improvement, methodology, query or suggestion
  7 ALERT type 5 Informative message, check
```

---

## Validation response form

Please find below a validation response form (VRF) that can be filled in and pasted into your CIF.

```
# start Validation Reply Form
_vrf_STRVA01_sm_621b
;
PROBLEM: Flack test results are ambiguous.
RESPONSE: ...
;
_vrf_PLAT220_sm_621b
;
PROBLEM: NonSolvent   Resd 1  C   Ueq(max)/Ueq(min) Range        4.7 Ratio
RESPONSE: ...
;
_vrf_PLAT242_sm_621b
;
PROBLEM: Low    'MainMol' Ueq as Compared to Neighbors of       N1SA Check
RESPONSE: ...
;
_vrf_PLAT911_sm_621b
;
PROBLEM: Missing FCF Refl Between Thmin & STh/L=    0.600         52 Report
RESPONSE: ...
;
# end Validation Reply Form
```

---

It is advisable to attempt to resolve as many as possible of the alerts in all categories. Often the minor alerts point to easily fixed oversights, errors and omissions in your CIF or refinement strategy, so attention to these fine details can be worthwhile. In order to resolve some of the more serious problems it may be necessary to carry out additional measurements or structure refinements. However, the purpose of your study may justify the reported deviations and the more serious of these should normally be commented upon in the discussion or experimental section of a paper or in the "special_details" fields of the CIF. checkCIF was carefully designed to identify outliers and unusual parameters, but every test has its limitations and alerts that are not important in a particular case may appear. Conversely, the absence of alerts does not guarantee there are no aspects of the results needing attention. It is up to the individual to critically assess their own results and, if necessary, seek expert advice.

**Publication of your CIF in IUCr journals**

A basic structural check has been run on your CIF. These basic checks will be run on all CIFs submitted for publication in IUCr journals (*Acta Crystallographica*, *Journal of Applied Crystallography*, *Journal of Synchrotron Radiation*); however, if you intend to submit to *Acta Crystallographica Section C* or *E* or *IUCrData*, you should make sure that full publication checks are run on the final version of your CIF prior to submission.

**Publication of your CIF in other journals**

Please refer to the *Notes for Authors* of the relevant journal for any special instructions relating to CIF submission.

---

**PLATON version of 02/02/2025; check.def file version of 02/02/2025**

**Datablock sm_621b** - ellipsoid plot

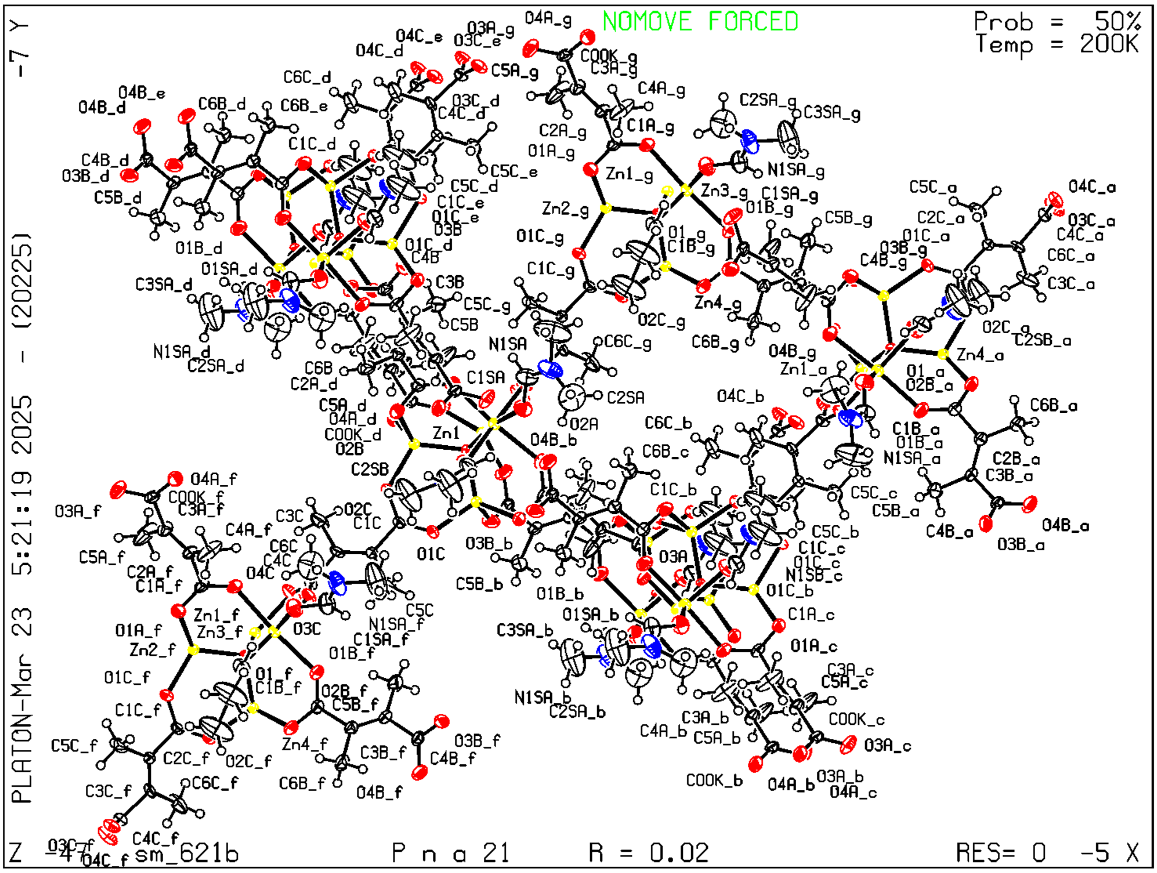

Supplement: Supplementary file 1 [file checkcif_AI-MOF-4.pdf]
